# Supplementary material for: Thermal fluctuations and carrier localization induced by dynamic disorder in MAPbI3 described by a first-principles based tight-binding model
Source: arXiv:2105.06525 source file (2021-07-19)
Supplement: Supplementary file 1 [file TB_Paper_Supplementary_Information.pdf]

# Supplementary Information for: Thermal fluctuations and carrier localization induced by dynamic disorder in $MAPbI_3$ described by a first-principles based tight-binding model

David J. Abramovitch
*Department of Physics, University of California, Berkeley*

Wissam A. Saidi
*Department of Mechanical Engineering and Materials Science, University of Pittsburgh*

Liang Z. Tan
*Molecular Foundry, Lawrence Berkeley National Laboratory*

## I. LATTICE PARAMETERS

Lattice parameters for the $\sqrt{2} \times 2 \times \sqrt{2}$ orthorhombic cell are given in Table I. Ratios between lattice parameter lengths are fixed based on experimental values (using the values of Baikie et [1] for the orthorhombic 150 K structure and Weller et al [2] for the tetragonal and cubic structures), and volumes are found by equilibrating in $6\sqrt{2} \times 12 \times 6\sqrt{2}$ unit cells with in the NPT ensemble. Additional trajectories used for tight binding are simulated using these lattice parameters with in the NVT ensemble.

| Temperature (K) | Lattice Constants (Å) | Volume ($Å^3$) | Structure |
|---|---|---|---|
| 150 K | ( 8.641 12.657 8.891) | 972.329 | orthorhombic |
| 220 K | ( 8.815 12.693 8.815) | 986.31 | tetragonal |
| 240 K | ( 8.824 12.689 8.824) | 988.073 | tetragonal |
| 260 K | ( 8.836 12.684 8.836) | 990.24 | tetragonal |
| 280 K | ( 8.848 12.675 8.848) | 992.248 | tetragonal |
| 300 K | ( 8.861 12.657 8.861) | 993.855 | tetragonal |
| 320 K | ( 8.878 12.633 8.878) | 995.842 | tetragonal |
| 340 K | ( 8.902 12.59 8.902) | 997.704 | cubic |

TABLE I. Lattice parameters for the $\sqrt{2} \times 2 \times \sqrt{2}$ unit cell as a function of temperature.

## II. COMPUTATIONAL METHODS

### A. Molecular Dynamics

Molecular dynamics atomic trajectories are obtained using the force field by Mattoni et al [3] in the LAMMPS molecular dynamics software [4] using the structures above. NVT ensemble is used for the generation of all tight binding trajectories, as explained above. We use a timestep of 0.5 fs.

### B. Potentials

Coulomb potentials and derivatives are found by a Ewald sum over atomic positions with the charges given in the main text. Length scales and cutoffs are chosen to converge the sum: a real space cutoff of 48 Å, reciprocal space cutoff of $\frac{2\pi}{8\mathring{A}}$ and a length scale to transition between real space and reciprocal space of 7.818 Å. Local potentials for each atomic species are calculated by a sum over neighboring atoms using the atomic radii in the main text. The sums are truncated at a cutoff length, with the cutoff length chosen to converge the calculation: 40 Åfor the sum over I atoms, 30 Åfor Pb, and 20 Åfor C, N, H-C, and H-N.

## III. COEFFICIENTS OF TIGHT BINDING FITS

In the equations for the fitting functions below, all energies are in eV, lengths are in Angstroms, Coulomb potentials ($V_C$) are in Volts, and short-range potentials ($V_{SR}$) have units of $\mathring{A}^{-3}$.

### A. Onsite Energies

Pb s onsite:

$$\begin{aligned}\epsilon_{\text{Pb s}} = &-0.2605546 * V_C - 0.0040925971 * (\frac{\partial^4}{\partial x^4}V_C + \frac{\partial^4}{\partial y^4}V_C + \frac{\partial^4}{\partial z^4}V_C) \\ &- 9490.4761 * V_{SR,Pb} + 48618.549 * \nabla^2 V_{SR,Pb} \\ &- 319.32019 * V_{SR,I} - 3180.4269 * \nabla^2 V_{SR,I} \\ &+ 7004.2506 * V_{SR,C} - 4652.5573 * \nabla^2 V_{SR,C} \\ &- 21193.459 * V_{SR,N} + 9486.0391 * \nabla^2 V_{SR,N} \\ &- 1448.9717 * V_{SR,H-c} + 606.52013 * \nabla^2 V_{SR,H-c} \\ &+ 7543.7332 * V_{SR,H-n} - 3029.378 * \nabla^2 V_{SR,H-n} \\ &- 9.9506426\end{aligned} \tag{1}$$

Pb p onsite:

$$\begin{aligned}\epsilon_{\text{Pb px}} = &-0.18627348 * V_C - 0.46838863 * \frac{\partial^2}{\partial x^2}V_C + 0.083344316\frac{\partial^4}{\partial x^4}V_C + 0.0096287899(\frac{\partial^4}{\partial y^4}V_C + \frac{\partial^4}{\partial z^4}V_C) \\ &- 11492.046 * V_{SR,Pb} + 45555.293 * \frac{\partial^2}{\partial x^2}V_{SR,Pb} + 47632.537 * (\frac{\partial^2}{\partial y^2} + \frac{\partial^2}{\partial z^2})V_{SR,Pb} \\ &+ 171.67848 * V_{SR,I} - 314.2043\frac{\partial^2}{\partial x^2}V_{SR,I} - 517.25294 * (\frac{\partial^2}{\partial y^2} + \frac{\partial^2}{\partial z^2})V_{SR,I} \\ &+ 2691.3918 * V_{SR,C} - 1946.4729\frac{\partial^2}{\partial x^2}V_{SR,C} - 1715.1296 * (\frac{\partial^2}{\partial y^2} + \frac{\partial^2}{\partial z^2})V_{SR,C} \\ &- 5466.395 * V_{SR,N} + 2366.2929\frac{\partial^2}{\partial x^2}V_{SR,N} + 2536.7662 * (\frac{\partial^2}{\partial y^2} + \frac{\partial^2}{\partial z^2})V_{SR,N} \\ &- 1811.3231 * V_{SR,H-c} + 705.12774\frac{\partial^2}{\partial x^2}V_{SR,H-c} - 697.73491 * (\frac{\partial^2}{\partial y^2} + \frac{\partial^2}{\partial z^2})V_{SR,H-c} \\ &+ 3143.7675 * V_{SR,H-n} - 1170.7807\frac{\partial^2}{\partial x^2}V_{SR,H-n} - 1301.7529 * (\frac{\partial^2}{\partial y^2} + \frac{\partial^2}{\partial z^2})V_{SR,H-n} \\ &- 3.9977575\end{aligned} \tag{2}$$

I p onsite:

$$\begin{aligned}
\epsilon_{\text{I px}} =& - 0.25267987 * V_C - 0.044231892 * \frac{\partial^2}{\partial x^2} V_C + 0.039340992 * \frac{\partial^4}{\partial x^4} V_C + 0.038408971 * (\frac{\partial^4}{\partial y^4} V_C + \frac{\partial^4}{\partial z^4} V_C) \\
& - 291.49742 * V_{SR,Pb} + 2057.0696 * \frac{\partial^2}{\partial x^2} V_{SR,Pb} + 1770.0459 * (\frac{\partial^2}{\partial y^2} + \frac{\partial^2}{\partial z^2}) V_{SR,Pb} \\
& + 407.31627 * V_{SR,I} + 3549.9385 * \frac{\partial^2}{\partial x^2} V_{SR,I} + 3683.7745 * (\frac{\partial^2}{\partial y^2} + \frac{\partial^2}{\partial z^2}) V_{SR,I} \\
& + 534.46694 * V_{SR,C} - 200.85386 * \frac{\partial^2}{\partial x^2} V_{SR,C} - 277.30551 * (\frac{\partial^2}{\partial y^2} + \frac{\partial^2}{\partial z^2}) V_{SR,C} \\
& + 3012.7269 * V_{SR,N} - 1090.9265 * \frac{\partial^2}{\partial x^2} V_{SR,N} - 1190.8312 * (\frac{\partial^2}{\partial y^2} + \frac{\partial^2}{\partial z^2}) V_{SR,N} \\
& + 9.2792723 * V_{SR,H-c} - 49.645418 * \frac{\partial^2}{\partial x^2} V_{SR,H-c} - 32.143503 * (\frac{\partial^2}{\partial y^2} + \frac{\partial^2}{\partial z^2}) V_{SR,H-c} \\
& - 112.12427 * V_{SR,H-n} - 53.279098 * \frac{\partial^2}{\partial x^2} V_{SR,H-n} - 18.060589 * (\frac{\partial^2}{\partial y^2} + \frac{\partial^2}{\partial z^2}) V_{SR,H-n} \\
& - 0.32580529 \delta_{\text{bond dir, p dir}} - 2.2947751
\end{aligned} \tag{3}$$

Where $\delta_{\text{bond dir, p dir}}$ is 1 if the orbital is in the direction of the Pb-I bond and 0 otherwise.

### B. Spin Orbit Coupling

In the equations for the spin-orbit coupling fitting functions below, $x$ and $y$ refer to the two orbitals in the hopping matrix element.

Pb p SOC:

$$\begin{aligned}
\gamma_{Pb} =& 0.046015007 * V_C + 0.061957126 * \frac{\partial^2}{\partial x^2} V_C + 0.069767544 * \frac{\partial^2}{\partial y^2} V_C \\
& + 0.034445864 * \frac{\partial^4}{\partial x^4} V_C + 0.034832375 * \frac{\partial^4}{\partial y^4} V_C - 0.0017593414 * \frac{\partial^4}{\partial z^4} V_C \\
& - 1361.0889 * V_{SR,Pb} + 4238.1026 * \frac{\partial^2}{\partial x^2} V_{SR,Pb} + 4290.9214 * \frac{\partial^2}{\partial y^2} V_{SR,Pb} + 5139.8108 * \frac{\partial^2}{\partial z^2} V_{SR,Pb} \\
& + 39.060802 * V_{SR,I} - 333.41433 * \frac{\partial^2}{\partial x^2} V_{SR,I} - 291.48468 * \frac{\partial^2}{\partial y^2} V_{SR,I} - 335.42281 * \frac{\partial^2}{\partial z^2} V_{SR,I} \\
& - 905.60705 * V_{SR,C} + 553.74013 * \frac{\partial^2}{\partial x^2} V_{SR,C} + 626.25846 * \frac{\partial^2}{\partial y^2} V_{SR,C} + 617.79812 * \frac{\partial^2}{\partial z^2} V_{SR,C} \\
& + 4131.3466 * V_{SR,N} - 1861.5942 * \frac{\partial^2}{\partial x^2} V_{SR,N} - 1924.176 * \frac{\partial^2}{\partial y^2} V_{SR,N} - 1668.6545 * \frac{\partial^2}{\partial z^2} V_{SR,N} \\
& - 147.58104 * V_{SR,H-c} + 56.055267 * \frac{\partial^2}{\partial x^2} V_{SR,H-c} + 38.456469 * \frac{\partial^2}{\partial y^2} V_{SR,H-c} + 45.356487 * \frac{\partial^2}{\partial z^2} V_{SR,H-c} \\
& - 1366.5571 * V_{SR,H-n}, 550.96036 * \frac{\partial^2}{\partial x^2} V_{SR,H-n} + 559.99982 * \frac{\partial^2}{\partial y^2} V_{SR,H-n} + 519.59972 * \frac{\partial^2}{\partial z^2} V_{SR,H-n} \\
& + 0.71444
\end{aligned} \tag{4}$$

I p SOC:

$$
\begin{aligned}
\gamma_I =& -9.780455 * 10^{-7} * V_C - 0.0060043296 * \frac{\partial^2}{\partial x^2} V_C - 0.0069648469 * \frac{\partial^2}{\partial y^2} V_C \\
& - 0.0015786324 * \frac{\partial^4}{\partial x^4} V_C - 0.0015662598 * \frac{\partial^4}{\partial y^4} V_C + 0.00045313142 * \frac{\partial^4}{\partial z^4} V_C \\
& + 13.793245 * V_{SR,Pb} + 14.416407 * \frac{\partial^2}{\partial x^2} V_{SR,Pb} + 16.201469 * \frac{\partial^2}{\partial y^2} V_{SR,Pb} + 3.0477232 * \frac{\partial^2}{\partial z^2} V_{SR,Pb} \\
& - 3.7663609 * V_{SR,I} + 5.6015585 * \frac{\partial^2}{\partial x^2} V_{SR,I} + 3.425553 * \frac{\partial^2}{\partial y^2} V_{SR,I} + 18.166615 * \frac{\partial^2}{\partial z^2} V_{SR,I} \\
& + 87.004756 * V_{SR,C} - 64.338737 * \frac{\partial^2}{\partial x^2} V_{SR,C} - 64.622115 * \frac{\partial^2}{\partial y^2} V_{SR,C} - 64.123072 * \frac{\partial^2}{\partial z^2} V_{SR,C} \\
& 113.23275 * V_{SR,N} - 48.521973 * \frac{\partial^2}{\partial x^2} V_{SR,N} - 47.859536 * \frac{\partial^2}{\partial y^2} V_{SR,N} - 52.754959 * \frac{\partial^2}{\partial z^2} V_{SR,N} \\
& - 11.483566 * V_{SR,H-c} + 5.2539584 * \frac{\partial^2}{\partial x^2} V_{SR,H-c} + 5.2902254 * \frac{\partial^2}{\partial y^2} V_{SR,H-c} + 5.420822 * \frac{\partial^2}{\partial z^2} V_{SR,H-c} \\
& - 5.5879105 * V_{SR,H-n} + 1.7585494 * \frac{\partial^2}{\partial x^2} V_{SR,H-n} + 1.7606195 * \frac{\partial^2}{\partial y^2} V_{SR,H-n} + 2.857072 * \frac{\partial^2}{\partial z^2} V_{SR,H-n} \\
& + 0.28880626
\end{aligned} \tag{5}
$$

### C. Bond and Non-Bonding Hopping

x is the direction of the bond, and y and z are perpendicular. For $\pi$ bonds, y is in the direction of the orbitals. For non-bonding, one orbital is the the x direction and one in the y direction. For hopping with $\pm$, the sign is determined by geometry, based on the positive and negative p-orbital lobes. It is + for Pb-I bonds in which the Iodine is in the positive direction from the Lead and - for bonds in the negative direction.
Pb s - I p $\sigma$ bond:

$$t_{sp,\sigma} = \pm 76.9763 * \exp(-1.3218 * x + 0.273781 * (y^2 + z^2)) - 0.129299 \tag{6}$$

Pb p - I p $\sigma$ bond:

$$t_{pp,\sigma} = 12.031 * \exp(-0.398815 * x + 0.111542 * (y^2 + z^2)) - 1.69694 \tag{7}$$

Pb s - I p $\sigma$ bond:

$$t_{pp,\pi} = -45.3656 * \exp(-1.46782 * x + 0.776221 * y^2 + 0.273144 * z^2) - 0.0343212 \tag{8}$$

Pb s - I p Nonbonding:

$$t_{sp,nb} = -93.0266 * y * \exp(-1.81299 * x - 0.25907 * z^2) \tag{9}$$

Pb p - I p Nonbonding:

$$t_{PbpIp,nb} = \pm 31.6277 * y * \exp(-1.24927 * x - 0.231421 * z^2) \tag{10}$$

I p - Pb p Nonbonding:

$$t_{IpPbp,nb} = \pm 34.7645 * y * \exp(-1.24836 * x - 0.186988 * z^2) \tag{11}$$

## IV. FULL MATRIX ELEMENT STATISTICS

Statistics for all matrix elements in the model are shown in Fig. 1, in addition to the subset shown in the main text.

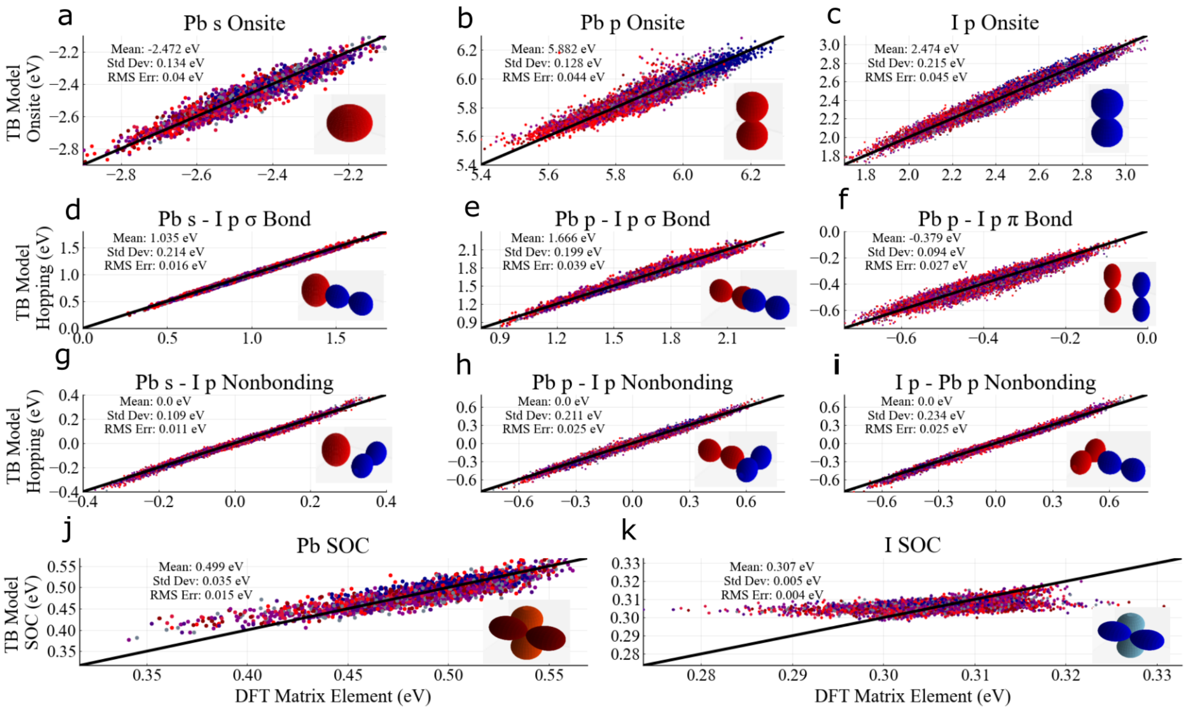


FIG. 1. Scatter plots and statistics for each matrix element in the tight binding model.

## V. ALTERNATE MATRIX ELEMENT FITS

To understand what physical processes influence different Hamiltonian matrix elements, it is informative to look at the accuracy of different fits. In the following tables, we compare different fits for onsite and hopping matrix elements.

Table V shows standard deviations and model RMS errors for the Pb s, Pb p, and I p onsite energies. It also shows the RMS error of the best fit using only Coulomb potentials (without local densities for each atomic species) and with no derivatives of the potentials (and therefore not differentiating p orbitals on the same atom). For p orbitals, the mean standard deviation of the instantaneous px, py, and pz orbital onsite energies on a given atom is also shown. Local potentials are shown to be very important, especially to I onsites in which they reduce the error by more than a factor of 2. Derivatives are shown to be very important to p orbitals, which can be understood by the large differences in p orbital energy on the same atom.

Table V shows standard deviation and model RMS errors for the bonding hopping parameters. It also shows the best fit RMS errors for a model using length only in the form $t_{ij} = a\exp\{(-r/b)\} + c$, as used by Mayers et al, and the best fit for a model in the form $t_0(\frac{r_0}{r})^2$, used by several authors, in which $t_0$ and $r_0$ are fitting parameters. The length only fit is shown to be quite accurate, although the direction specific fits used in our model offer a modest improvement. The $t_0(\frac{r_0}{r})^2$ fit does not very accurately fit our data.

| Orbital | Onsite SD (eV) | Model RMS Err (eV) | Coulomb Only RMS Err (eV) | No Derivatives RMS Err (eV) | Mean Single Atom px, py, pz SD (eV) |
|---|---|---|---|---|---|
| Pb s | 0.1341 | 0.0405 | 0.0670 | 0.0462 | |
| Pb p | 0.1284 | 0.0441 | 0.0767 | 0.0934 | 0.0898 |
| I p | 0.2153 | 0.0454 | 0.1056 | 0.1219 | 0.1253 |

TABLE II. Statistics comparing alternative onsite energy fits. Model refers to the complete tight binding model, Coulomb only refers to a least squares fit excluding local potential effects, and no derivatives refers to a least squares fit excluding directional derivatives of potentials.

| Bond | Hopping SD (eV) | Model RMS Err (eV) | Length Only RMS Err (eV) | $t_0(\frac{r_0}{r})^2$ RMS Err (eV) |
|---|---|---|---|---|
| sp $\sigma$ | 0.2143 | 0.0163 | 0.0199 | 0.1245 |
| pp $\sigma$ | 0.1993 | 0.0390 | 0.0473 | 0.0684 |
| pp $\pi$ | 0.0937 | 0.0269 | 0.0370 | 0.0646 |

TABLE III. Statistics comparing alternative hopping parameter fits. Length only $(a\exp\{(-r/b)\}+c)$ and $t_0(\frac{r_0}{r})^2$ fits show the best fits in that form as a function of the bond length $r$ and fitting variables $a$, $b$, $c$, $t_0$, and $r_0$.

## VI. STATISTICAL DISTRIBUTIONS OF MATRIX ELEMENTS AT FINITE TEMPERATURE

To understand the fluctuations in the different Hamiltonian matrix elements, it is informative to look at statistical distributions for each Hamiltonian matrix element. Distributions for onsite and hopping matrix elements are shown in Fig. 2 and distributions for spin orbit coupling matrix elements are shown in Fig. 3

It is noteworthy that standard deviation of many matrix elements only increases a small amount with temperature. This indicates that much of the variation in Hamiltonian matrix elements comes from low frequency dynamic disorder, which is only weakly temperature dependent, as discussed in the main text.

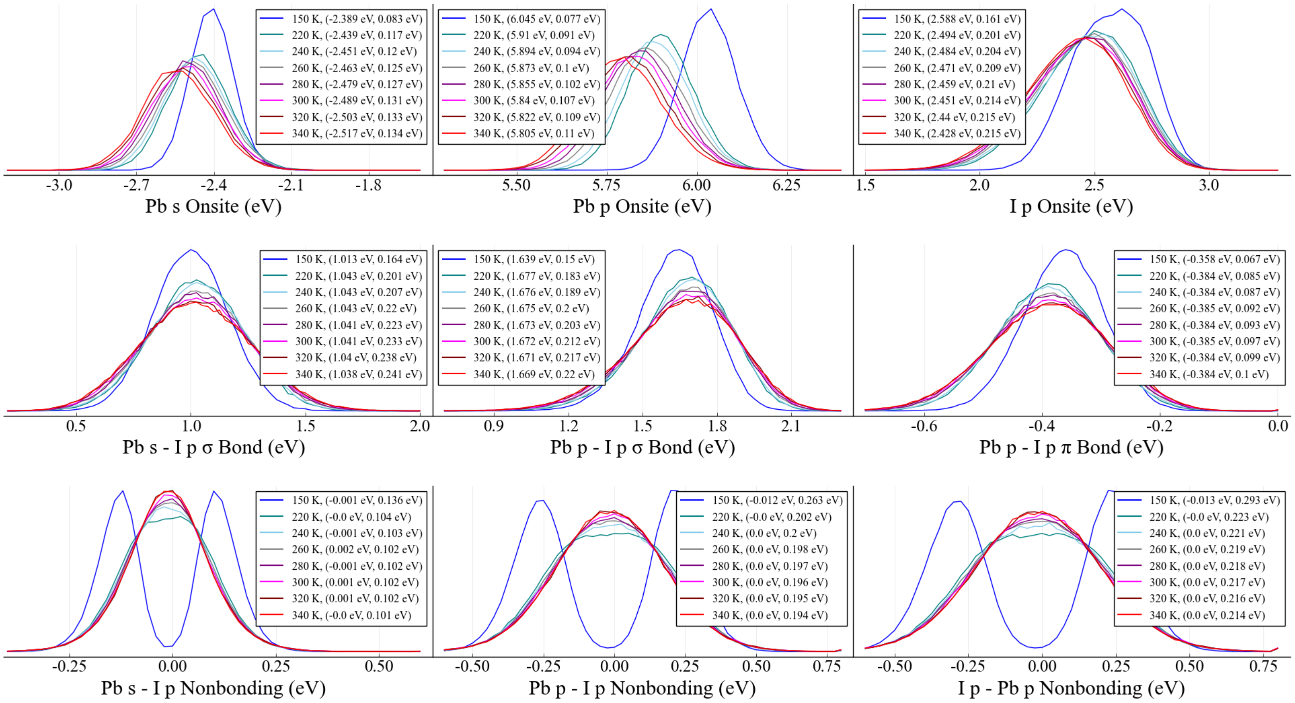


FIG. 2. Statistical distributions of onsite and hopping matrix elements computed from 2000 $2 \times 2 \times 2$ structures at each temperature. Mean and standard deviation are given in parentheses for each temperature.

## VII. ACCURACY OF TIGHT BINDING IN ORTHORHOMBIC STRUCTURE

In the main text, benchmarks on the tight binding model focus on the orthogonal and tetragonal temperatures of 220 - 340 K. Comparisons including orthorhombic (150 K) structures in Fig. 4 show generally good results as well, however the 150 K structure shows a somewhat overestimated bandgap and electron and hole masses. Fluctuations, however, are generally predicted well.

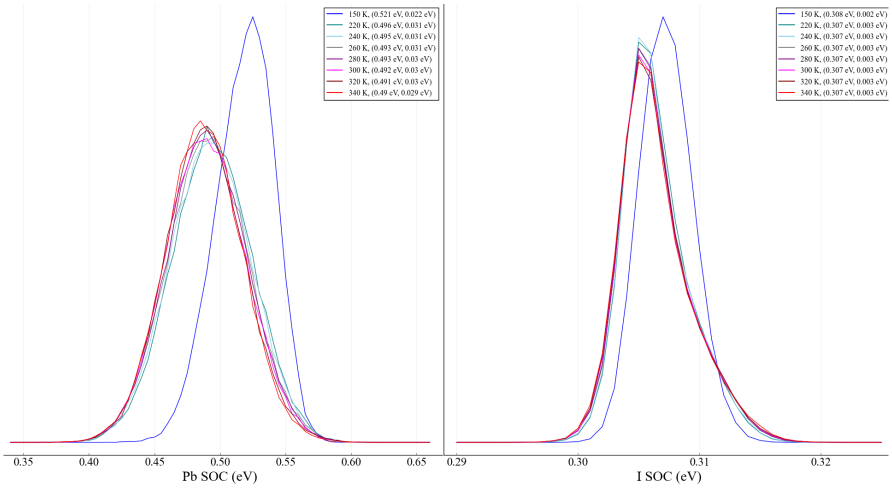


FIG. 3. Statistical distributions of spin orbit coupling matrix elements computed from 2000 2 x 2 x 2 structures at each temperature.

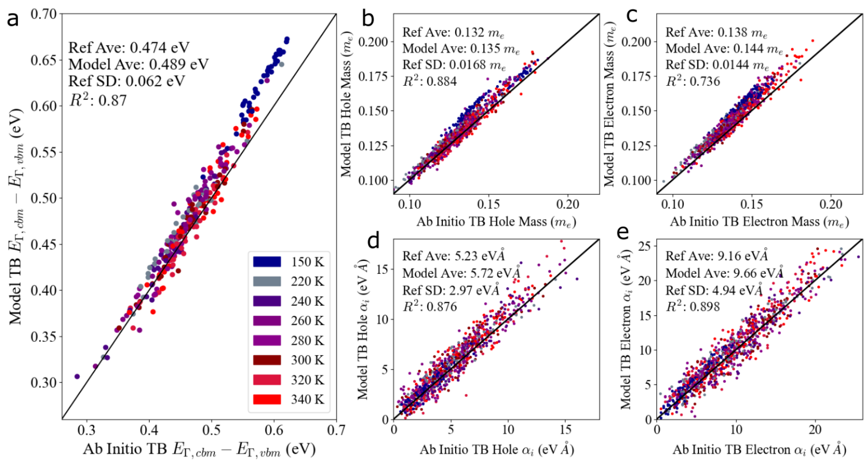


FIG. 4. Tight binding model predictions of (a) bandgap, (b) hole and (c) electron mass, and (d) valence and (e) conduction band spin splitting, including temperatures 150-340 K.

## VIII. ACCURACY OF TIGHT BINDING COMPARED TO DFT

The tight binding model uses a restricted set of matrix elements, which are each individually fitted to DFT calculated matrix elements. To evaluate the accuracy of this restricted matrix element set, we compare its predictions to full planewave DFT, which effectively include all matrix elements. We compare the model prediction of Γ point energy gap, carrier mass, and spin splitting to DFT. We find that the model predicts trends in these quantities well compared to full planewave DFT ( Figure 5). While there are some systematic errors including overestimating bandgap and electron mass and underestimating spin splitting, the trends are predicted well, indicating that the thermal fluctuations in these quantities have been captured by the distance-dependence of the model. Additionally, a comparison with Figure 6 shows that the current model represents a large increase in accuracy, in both mean values and fluctuations, compared to previous models Ref. [5].

## IX. EFFECT OF MODEL COMPONENTS, SIMPLIFIED MODELS

We plot the predictions of bandgap, electron and hole mass, and valence and conduction band spin splitting with four simplified models, demonstrating the importance of different components. Each of the four simplified models has one

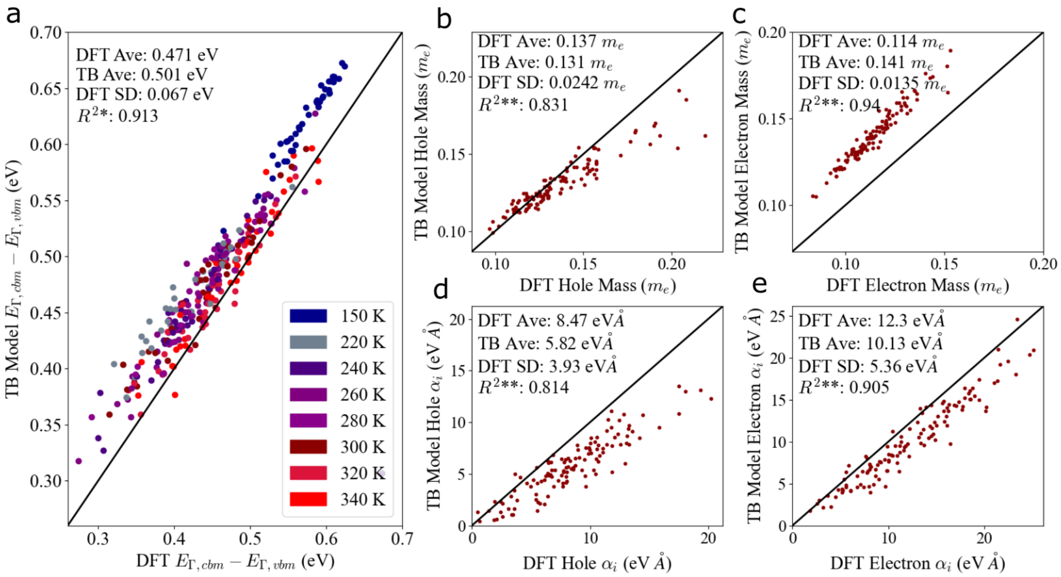


FIG. 5. TB model band structure predictions compared to DFT. The model predicts fluctuations $\Gamma$ point energy gap well, though it systematically overestimates bandgaps by about 0.03 eV. The model also systematically overestimates electron mass by about 24 % and underestimates spin splitting by about by about 31% for holes and 18% for electrons. $R^{2*}$ value allows for a constant offset between DFT and tight binding values. $R^{2**}$ value allows for a constant multiplicative factor between DFT and tight binding values.

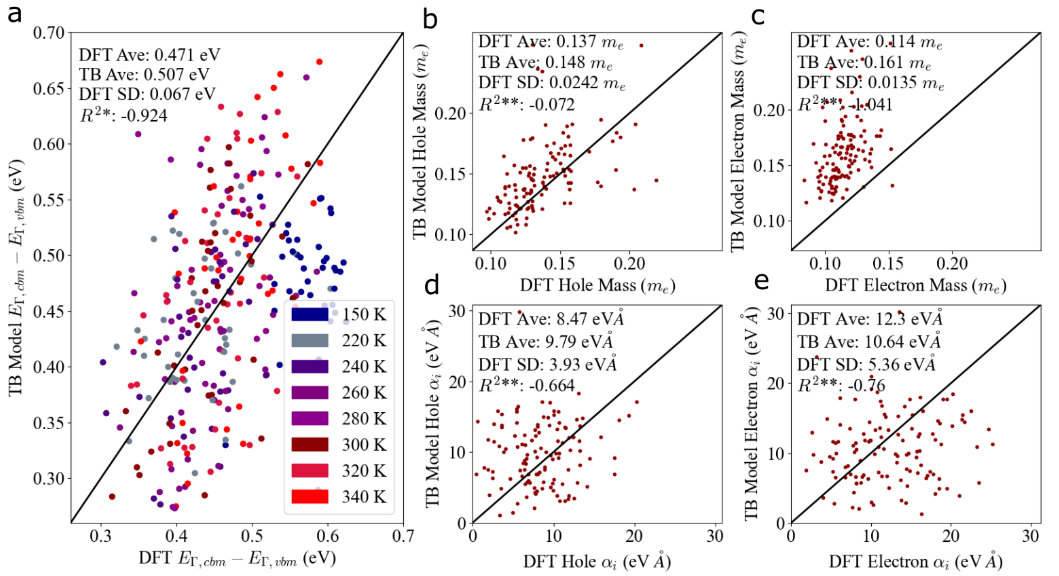


FIG. 6. Previous TB model [5] $\Gamma$ point energy gap compared to DFT. $R^{2*}$ value allows for a constant offset between DFT and tight binding values. $R^{2**}$ value allows for a constant multiplicative factor between DFT and tight binding values

modification from the physical model: constant onsite energies, constant bond hopping parameters, no non-bonding hopping parameters, and constant spin orbit coupling hopping parameters.

Through these calculations, we can assess the effects of different fluctuations. Onsite energy fluctuations play a significant role in bandgap fluctuations, as well as lowering the bandgap compare to constant onsite energies. This can be rationalized VBM (CBM) states disproportionately occupy the highest (lowest) energy orbitals. Onsite fluctuations also appear to lower the carrier mass, likely linked to the bandgap renormalization. Bond fluctuations play an important role in onsite fluctuations, mass fluctuations, and spin splitting. though they appear to have a

smaller effect on averages. Non-bonding matrix elements, which in the tetragonal and cubic structures originate completely from fluctuations, play an important role in the bandgap fluctuations and spin splitting, increasing the bandgap. Spin orbit coupling fluctuations appear to play a smaller role, but affect bandgap fluctuations, in particular comparing the orthorhombic and tetragonal structures.

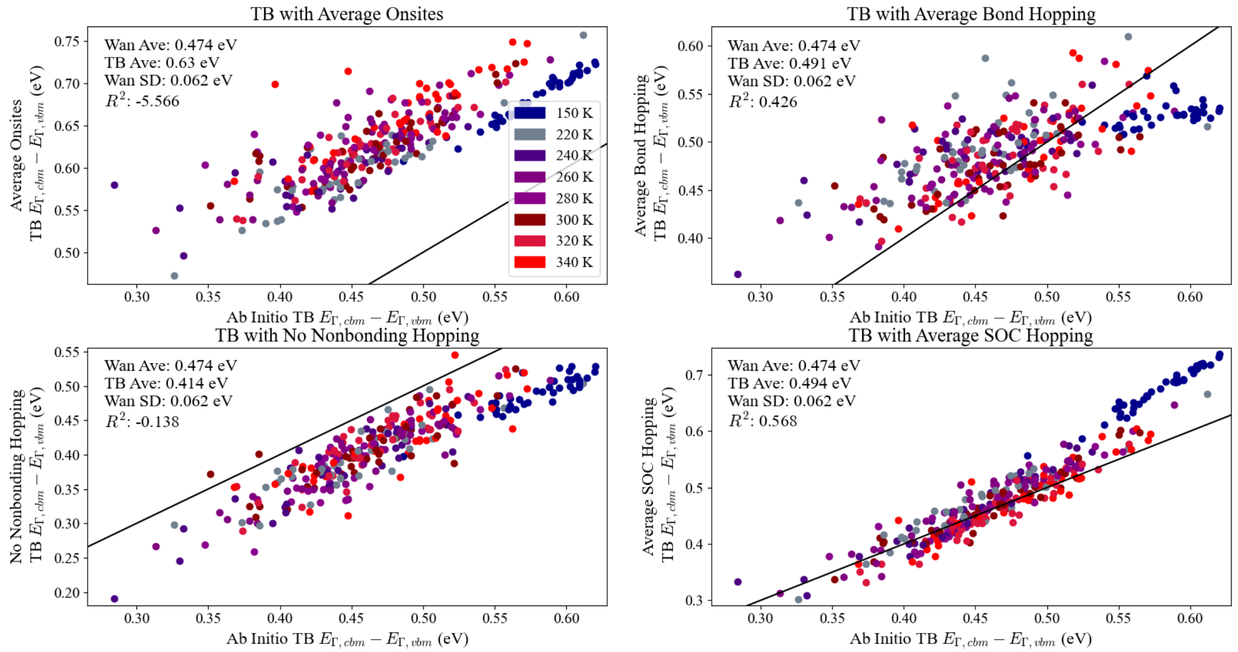


FIG. 7. Prediction of bandgap fluctuations with 4 simplified models.

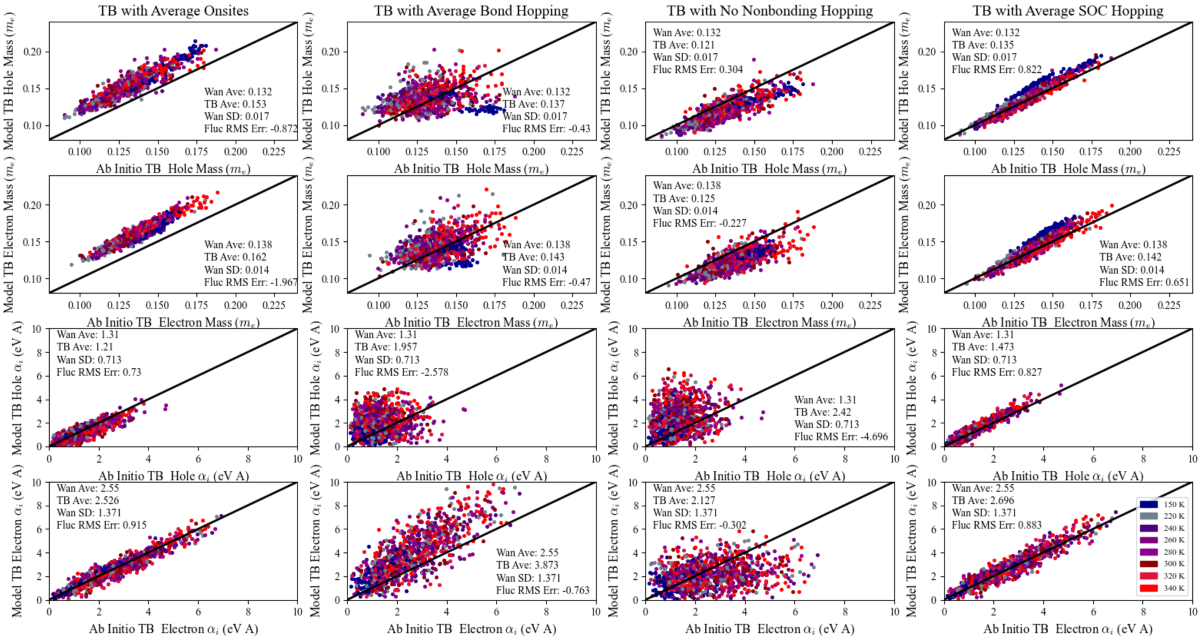


FIG. 8. Prediction of electron and hole mass and valence and conduction band spin splitting with 4 simplified models. Bonding and non-bonding hopping parameters play the most important role, consistent with hopping matrix elements representing dispersion and non-bonding and bond fluctuations breaking inversion symmetry.

[1] T. Baikie, Y. Fang, J. M. Kadro, M. Schreyer, F. Wei, S. G. Mhaisalkar, M. Graetzel, and T. J. White, Synthesis and crystal chemistry of the hybrid perovskite (ch3nh3)pbi3 for solid-state sensitised solar cell applications, J. Mater. Chem. A **1**, 5628 (2013).

[2] M. T. Weller, O. J. Weber, P. F. Henry, A. M. Di Pumpo, and T. C. Hansen, Complete structure and cation orientation in the perovskite photovoltaic methylammonium lead iodide between 100 and 352 k, Chem. Commun. **51**, 4180 (2015).

[3] A. Mattoni, A. Filippetti, M. I. Saba, and P. Delugas, Methylammonium rotational dynamics in lead halide perovskite by classical molecular dynamics: The role of temperature, The Journal of Physical Chemistry C **119**, 17421 (2015), https://doi.org/10.1021/acs.jpcc.5b04283.

[4] S. Plimpton, Fast parallel algorithms for short-range molecular dynamics, Journal of Computational Physics **117**, 1 (1995).

[5] M. Z. Mayers, L. Z. Tan, D. A. Egger, A. M. Rappe, and D. R. Reichman, How lattice and charge fluctuations control carrier dynamics in halide perovskites, Nano Letters **18**, 8041 (2018), pMID: 30387614, https://doi.org/10.1021/acs.nanolett.8b04276.
